# Supplementary material for: Towards Open-Set Test-Time Adaptation Utilizing the Wisdom of Crowds in Entropy Minimization
Source: arXiv:2308.06879 source file (2023-09-04)
Supplement: Supplementary file 1 [file supple_open.tex]

%#################################################################################################
\begin{table}[t]
\centering
%#################################################
% Rounds 100
%#################################################
\begin{center}
{\resizebox{0.47\textwidth}{!}{
{
\begin{tabular}{c|ccc} 
\toprule
Method & 0.2 & 0.5 & 0.8  \\ 
\toprule
Source~\cite{wrn} & 18.27 & 18.27 & 46.75 \\
BN Adapt~\cite{tbn} & 14.42 & 15.73 & 17.67  \\
\hline
TENT~\cite{tent} & 63.19 & 85.22 & 84.77 \\
\rowcolor{Gray}+ Ours & \textbf{14.16 (-49.03)} & \textbf{15.77 (-69.45)} & \textbf{18.14 (-66.63)} \\
\hline
% EATA~\cite{tent} & 77.78 & 82.05 & 84.23  \\
% \rowcolor{Gray}+ Ours & \textbf{14.20 (-63.58)} & \textbf{15.65 (-66.40)} & \textbf{18.27 (-65.96)} \\
% \hline
SWR~\cite{tent} & 90.14 & 90.55 & \textbf{87.37}  \\
\rowcolor{Gray}+ Ours & \textbf{23.85 (-66.29)} & \textbf{72.58 (-17.97)} & 89.43 (+2.06) \\
\hline
\toprule
\end{tabular}}}}
\end{center}
\vspace{-0.5cm}
\caption{Open-set TTA performances with diverse ratios of open-set samples.}
\vspace{-0.3cm}
\label{tab:supple_open_diverse}
\end{table}
%##################################################################################################
