# Supplementary material for: Towards Open-Set Test-Time Adaptation Utilizing the Wisdom of Crowds in Entropy Minimization
Source: arXiv:2308.06879 source file (2023-09-04)
Supplement: Supplementary file 2 [file supple_threshold.tex]

\begin{table*}[t]
\centering
%#################################################
% Rounds 50
%#################################################
\begin{center}
{\resizebox{0.8\textwidth}{!}{
{
\begin{tabular}{c|ccc|ccc} 
\toprule
\multirow{2}{*}{Threshold} & \multicolumn{3}{c|}{CIFAR-10-C}  & \multicolumn{3}{c}{CIFAR-100-C} \\
       & Precision (\%) & Recall (\%) & F1-score & Precision (\%) & Recall (\%) & F1-score \\ 
\toprule
0.5 & 55.65 &\textbf{1.00} & 0.02 & 54.59 & \textbf{99.89} & 0.71 \\
0.8 & 55.92 & 99.08 & 0.71 & 56.17 & 97.49 & 0.71 \\
0.9 & 63.72	& 99.03 & 0.78 & 58.94 & 95.49 & 0.73 \\
0.95 & 53.54 & 98.22 & 0.69 & 59.58 & 92.90 & 0.73 \\
0.99 & 53.37 & 97.56 & 0.69 & 59.52 & 90.83 & 0.72 \\
Entropy~\cite{eata} & 59.98 & 99.98 & 0.75 & 58.46 & 95.31 & 0.72 \\
\rowcolor{Gray} Ours & \textbf{85.54} & 96.90 & \textbf{0.91} & xxxx & xxxx & xxxx \\
\toprule
\end{tabular}}}}
\end{center}
\vspace{-0.6cm}
\caption{Comparisons on precision and recall with various thresholds.}
\label{tab:supple_threshold} 
\vspace{-0.1cm}
\end{table*}
%##################################################################################################
